# Supplementary material for: Electrical tuning of helical edge states in topological multilayers
Source: arXiv:1903.02687 ancillary file (2019-07-22)
Supplement: Supplementary file 1 [file SuppMat.pdf]

# Supplementary Material: Electrical tuning of helical edge states in topological multilayers

**T. Campos[1,4], M. A. Toloza Sandoval[2], L. Diago-Cisneros[3,4], G. M. Sipahi[4]**

[1] Department of Physics, State University of New York at Buffalo, Buffalo, New York 14260, USA
[2] Instituto de Física, Universidade Federal da Bahia, Salvador, Bahia 40210-340, Brazil.
[3] Facultad de Física, Universidad de La Habana, La Habana 10400, Cuba
[4] Instituto de Física de São Carlos, Universidade de São Paulo, São Carlos, São Paulo 13566-590, Brazil

## Oscillatory decaying edge states

Following Ref. [1] the oscillations in the probability densities of the edges states can be understood by a simple mathematical argument. Using the ansatz, $\Psi(x) \propto e^{\lambda x}$, for the wave function of the edge states we can solve the BHZ model [2] for $\lambda$ in the middle of the gap to find

$$\lambda = \pm \left( \frac{A}{2\sqrt{B^2 - D^2}} \pm i \sqrt{\frac{M}{B} - \frac{A^2}{4\,(B^2 - D^2)}} \right) \qquad (1)$$

When $\frac{M}{B} - \frac{A^2}{4(B^2-D^2)} > 0$, $\lambda$ has a nonzero imaginary part which yields the oscillations. The parameters $A$, $B$, $D$ and $M$ are system specific and are found following Ref. [2], we did not derive any of these parameters in this study since it is outside of the scope.

## Semiconductor-Semimetal transition

In this section we discuss the semiconductor-semimetal transition for the broken gap quantum wells.

*Asymmetric quantum well*

In figure 1 we show the semiconductor-semimetal transition for the InAs/GaSb asymmetric quantum well (AQW). In figure 1(a) and figure 1(b) the system is still in the semiconductor phase. To be in the semiconductor phase means that, at the Γ-point, the bottom of the conduction band is still above the top of the valence band. As we increase the size of the InAs layer we are decreasing the electron's quantum confinement and, therefore, its energy level decreases – asymptotically to the bottom of the conduction band. Since the top of the valence band is above to bottom of the conduction band, there will be a size when the electron energy level crosses below the holes energy level. [3, 4] In figure 1(c) and figure 1(d) we show the band structure of the system when the electron energy level is far bellow the holes energy level. In this case, we characterize the system as in a semimetal phase. Notice that there is no overall gap in such a configuration. Even though, for select cases, such as the one in figure 1(c), there is still a hybridization gap along [100] direction, due to the asymmetries of the valence band, this hybridization gap vanishes along [110] direction making the system gapless.

*Symmetric quantum well*

For symmetric quantum wells (SQW) the semiconductor-semimetal transition is different of the AQW on and can be characterized in two cases [5, 6]. First, for the case of InAs/GaSb/InAs symmetric quantum well, the system has two electron subbands lying in the broken gap region. As we change the sizes of the InAs layer, these electrons subbands shift in energy but only one subband interacts with the HH subband while the other stay still. Furthermore, since the SQW does not have a intrinsic Rashba SOC, there is no hybridization gap. In figure 2(a) the system is in the semiconductor phase, while in the case of figure 2(b) and figure 2(c) the system is in the semi-metal phase. The case of figure 2(b) can be seen as a transition state where the system does not have a overall gap because the top of the valence band occurs at a finite $k$ wave vector while the bottom of the conduction band is on the Γ-point. Increasing the size of the InAs layer makes one of the electron subbands penetrates deep in the valence subbands state but anticrossing them, see figure 2(c).

For the case of the the GaSb/InAs/GaSb SQW, figure 2(d)-(f), we have that the system has now only one type of electron subband while two types of holes subbands. In this case, the system depicted in figure 2(d) is in the semiconductor phase. By change the size of the active layers we can see that an interesting configuration of the subbands appear. Take, for instance, figure 2(e), where the lowest electron subband almost touches the holes subbands. In this situation, the system is still in the semiconductor phase – since there is no inversion of the bands – but the overall gap is almost vanishing. By tuning the size of the active layers we can make the system have a degenerate electron and hole state at the Γ-point. Increasing the sizes of the active layers we can drive the system to a semi-metal phase, see figure 2(f), but interesting enough both electron and one of the HH subbands remains degenerate in a region around Γ-point, while the hybridization occurs with lower lying hole subbands.

## InAs/GaSb Asymmetric QWs

In figure 3 we show the hybridization gap heatmap of the InAs/GaSb AQW. Figure 3(a) shows the general flat band profile with the InAs/GaSb active region surrounded by a AlSb barrier. In such a configuration,

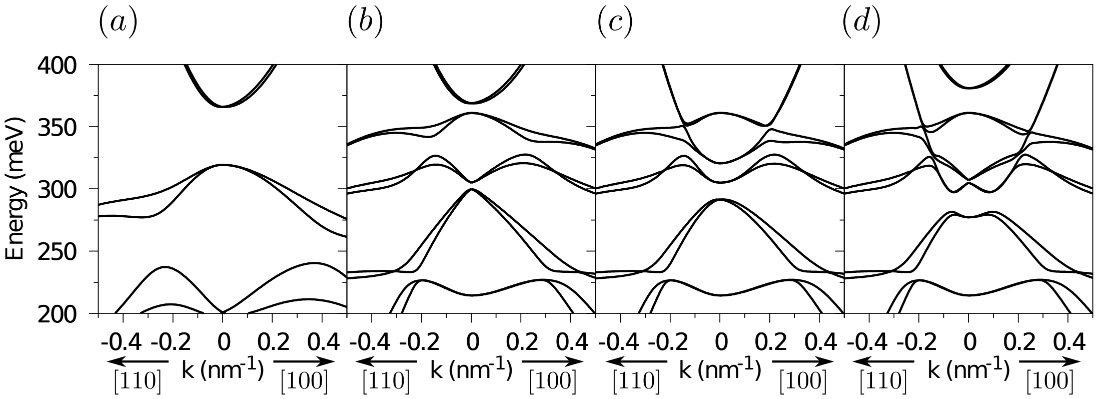


**Figure 1.** Semiconductor-semimetal transition of InAs/GaSb asymmetric quantum well. (a) is for layer length $L_{\text{GaSb}} = 4\,\text{nm}$ and $L_{\text{InAs}} = 8\,\text{nm}$, (b) $L_{\text{GaSb}} = 8\,\text{nm}$ and $L_{\text{InAs}} = 8\,\text{nm}$, (c) for $L_{\text{GaSb}} = 8\,\text{nm}$ and $L_{\text{InAs}} = 12\,\text{nm}$ and (f) for $L_{\text{GaSb}} = 8\,\text{nm}$ and $L_{\text{InAs}} = 16\,\text{nm}$. (a) and (b) shows the band structure for the case were the system is in the semiconductor phase. (c) and (d) shows the band structure were the system is in the semi-metal phase. In this case, all subbands are spin-split.

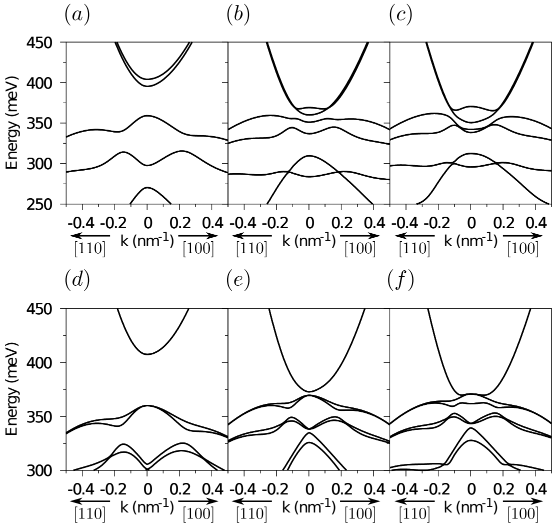


**Figure 2.** Semiconductor-semimetal transition of symmetric quantum well. (a) and (d) are for layer length $L_{\text{GaSb}} = 8\,\text{nm}$ and $L_{\text{InAs}} = 7\,\text{nm}$, (b) and (e) for $L_{\text{GaSb}} = 11\,\text{nm}$ and $L_{\text{InAs}} = 9\,\text{nm}$, (c) and (f) for $L_{\text{GaSb}} = 12\,\text{nm}$ and $L_{\text{InAs}} = 10\,\text{nm}$. (a), (b) and (c) are the band structure for the case of the InAs/GaSb/InAs QW and (d), (e) and (f) are the band structure of the GaSb/InAs/GaSb QW. In both cases, the subbands are spin degenerated.

the electrons stay confined in the InAs layer while the holes stay in the GaSb layer. By controlling the lengths of the active layers it is possible to drive the system from a insulating regime – when the energy of the electrons stay above the energy of the holes – to a inverted, hybridized, regime – when the holes' energy crosses the electrons' energy [7, 4, 8]. In the inverted regime, the main physical quantity which characterize the system is the hybridization gap, $\Delta E_h$, defined as the energy gap which opens due to the spin-orbit coupling in a non-zero $k$ vector. By applying an electric field along the confinement direction we can tune the strength of the spin-orbit coupling and, therefore, the magnitude of $\Delta E_h$ [9, 10].

In figure 3(b), figure 3(d) and 3(f) we show the complete phase diagram of the hybridization gap as a function of the sizes of the active layers (InAs and GaSb) for the most common studied samples [11, 12, 13, 14, 15, 16, 17, 18, 19, 20, 21, 22, 23, 24, 25, 26, 27, 28]. By varying the electric field from $E = -5\,\text{mV}\,\text{nm}^{-1}$, figure 3(b), to $E = 5\,\text{mV}\,\text{nm}^{-1}$, figure 3(f), we see that the hybridization gap increases about 2 meV. Furthermore, for negative electric fields the hybridization occurs for larger sizes of the active layers and as we increase the magnitude of the electric field the hybridization tends to occur for smaller sizes of the active layers. Take for example the case without electric field, figure 3(d), we see that the hybridization gap occurs in the middle of the phase diagram with maximum value around $\Delta E_h \approx 4.5\,\text{meV}$, as reported previously in the literature [26].

In figure 3(c), figure 3(e) and figure 3(g) we show the band structure and the component polarized DOS for a select representative QW, marked as a star in figure 3(b), figure 3(d) and figure 3(f), respectively. We plotted the band structure as a function of all $k_{\|}$ setting $k = \sqrt{k_x^2 + k_y^2}$. Doing this, we access all the information about the anisotropy of the valence band dispersion. We computed the hybridization gap, $\Delta E_h$, by calculating the energy of the region where there is no DOS, therefore $\Delta E_h$ is the overall hybridization gap taking into account all the features of the band structure, see Supplemental Material. Moreover, the hybridization gap is only defined for systems where the HH DOS exists in the energy range of the electrons. If there is no HH DOS in the electron energy range the QW is in the insulator regime, and if there is to much penetration of the electron and holes the hybridization gap collapses and the system becomes

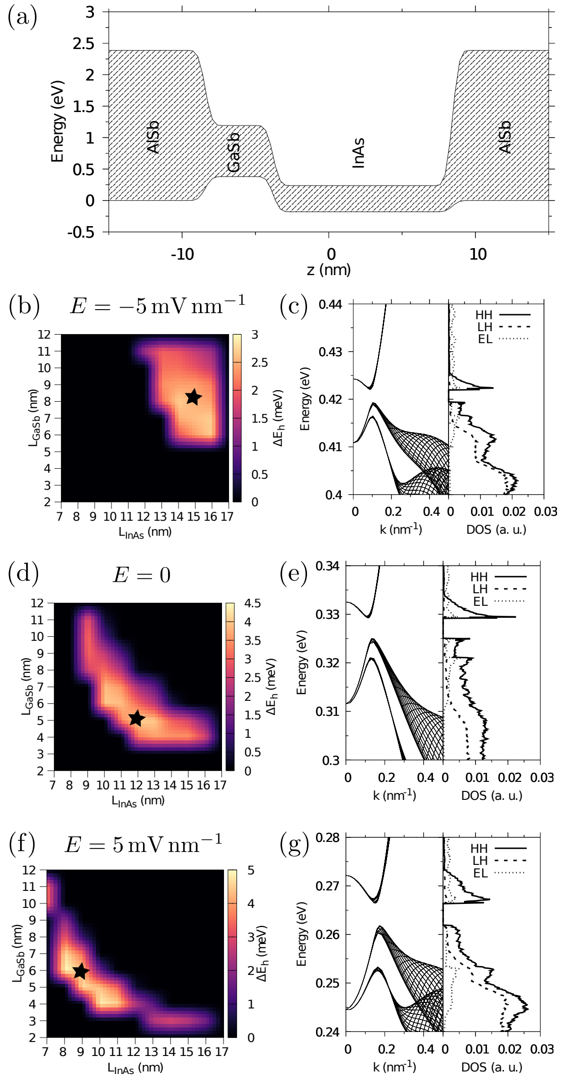


**Figure 3.** Hybridization gap heatmap of the InAs/GaSb AQW. (a) Flat band profile for the AQW. (b), (d) and (f) hybridization gap heat map of AQW as function of the InAs and GaSb layer sizes: (b) with an applied electric field of $E = -5\,\mathrm{mV\,nm^{-1}}$, (d) $E = 0$ and (f) $E = 5\,\mathrm{mV\,nm^{-1}}$. (c) band structure and polarized DOS for the AQW with $L_{\mathrm{GaSb}} = 8\,\mathrm{nm}$ and $L_{\mathrm{InAs}} = 15\,\mathrm{nm}$ and an applied electric field of $E = -5\,\mathrm{mV\,nm^{-1}}$. (e) band structure and polarized DOS for the AQW with $L_{\mathrm{GaSb}} = 5\,\mathrm{nm}$ and $L_{\mathrm{InAs}} = 12\,\mathrm{nm}$ without an applied electric field. (g) band structure and polarized DOS for the AQW with $L_{\mathrm{GaSb}} = 6\,\mathrm{nm}$ and $L_{\mathrm{InAs}} = 9\,\mathrm{nm}$ and an applied electric field of $E = 5\,\mathrm{mV\,nm^{-1}}$. The wave vector $k$ in (c), (e) and (g) is defined as $k = \sqrt{k_x^2 + k_y^2}$. The star in (b), (d) and (f) represent the point where the band structure and DOS were computed. From negative to positive electric field the hybridization gap $k$ value increases and also the maximum value of $\Delta E_h$ increased about 2 meV.

a semimetal [3, 7, 4, 29, 30, 27]. Furthermore, it is also possible to see that for negative electric fields the $k$-point where the hybridization occurs is closer to the $\Gamma$-point than for positive electric fields. This means that based on the estimation of the Fermi velocity as $v_F \approx \frac{\Delta E_h}{2\hbar k_c}$, where $k_c$ is the wave vector value were the crossing occurs, for increasingly positive electric field the system becomes more and more interacting [10, 31].

Also in figure 3(c), figure 3(e) and figure 3(g) we can see that the two spin-split subbands bellow the hybridization gap have a anomalous (or giant) spin-split as previously stated in the literature [11, 12, 25, 32]. Although this feature is beyond the scope of this manuscript, it is worthwhile mention.

## Edge State Probability Densities: InAs/GaSb Asymmetric QWs

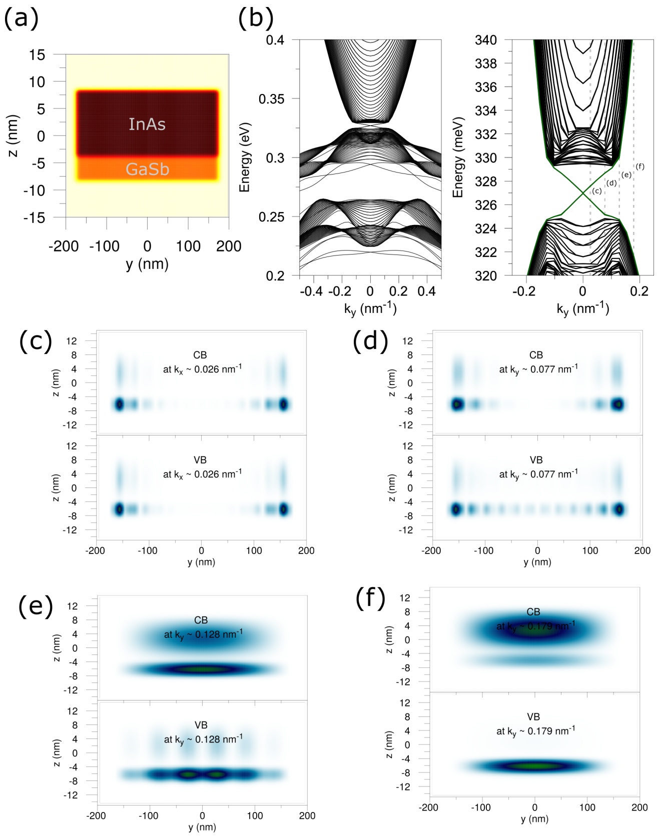


**Figure 4.** Energy dispersion and edge states probability densities with $E = 0$ for a $L_{\mathrm{GaSb}} = 5\,\mathrm{nm}$ and $L_{\mathrm{InAs}} = 12\,\mathrm{nm}$ AQW. (a) Flat band profile for the slab with the $z$ axis being the quantum well growth direction and the $y$ axis the slab confinement, the $x$ axis is assumed to have periodic boundary condition. (b) Zoom out energy dispersion of the slab on the left and zoomed energy dispersion focused on the region where the Dirac cone should be. (c)-(f) are the probability densities, for the conduction band on the top panel and valence band on the bottom panel, of the edge states at the wave vector depicted on (b).

In figure 4(a) we show the flat band confinement profile of the InAs/GaSb slab with $L_{\mathrm{GaSb}} = 5\,\mathrm{nm}$ and $L_{\mathrm{InAs}} = 12\,\mathrm{nm}$ in the $zy$-plane, while the $x$ direction have periodic boundary condition, without

an applied electric field. In figure 4(b) we show the zoom out energy dispersion, on the left panel, and on the right panel the zoom in around the Dirac cone. In figure 4(c)-(f) we show the probability densities of the edge states. In figure 4(c) we see that, near the Γ-point, the states are very localize near the edge, with a small oscillating tail. At $k_y \approx 0.077\,\mathrm{nm}^-1$ the valence edge state start delocalize, see figure 4(d). Increasing the wave vector, the states are now localized at the center of the profile indicating that they are becoming more like bulk states than edge states, see figure 4(e). At a wave vector outside the Dirac cone region the states are now, indeed, bulk like: the conduction state is localized at the InAs layer while the valence at the GaSb.

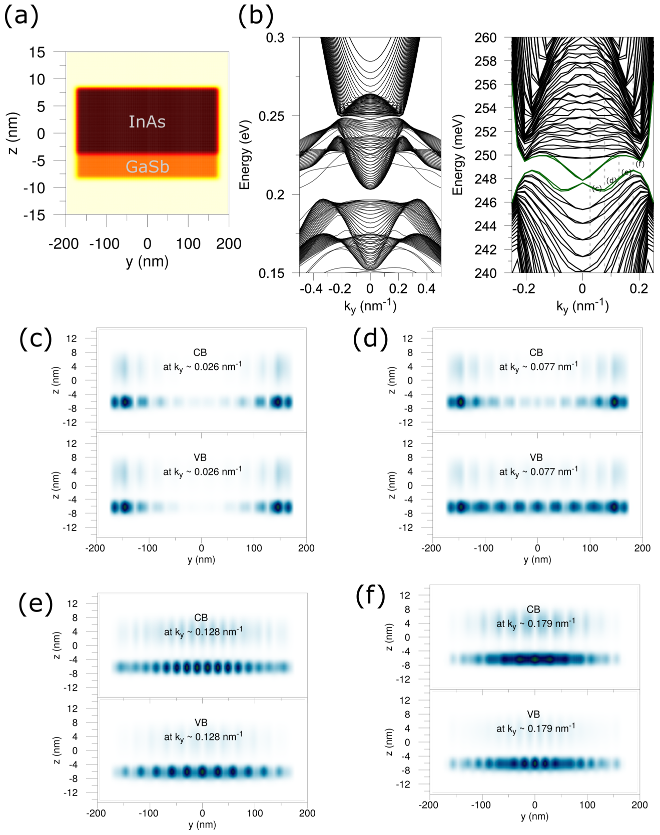


**Figure 5.** Same as figure 4 but with $E = 5\,\mathrm{mV\,nm}^{-1}$.

The robustness of the edge states observed experimentally [17] is attributed to the burring of the Dirac cone inside the valence band subbands [26, 28]. By either changing the size of the active layers or by applying an electric field we can engineer a system with this property. In figure 5 we show such a case were the Dirac cone is hidden by the application of an electric field. In figure 5(a) we show the flat band confinement profile of the InAs/GaSb slab with $L_{\mathrm{GaSb}} = 5\,\mathrm{nm}$ and $L_{\mathrm{InAs}} = 12\,\mathrm{nm}$ in the $zy$-plane. In figure 5(b) its energy dispersion were it becomes clear that the Dirac cone is hidden. Such a system is in a strongly interacting regime, which can be seen by the probability densities of the edge states. In figure 5(c) we already see that both conduction and valence edge states are oscillating with a tail. Increasing the wave vector only makes this feature more pronounced, as seen throughout figure 5(d)-(f). This system is very similar to the GaSb/InAs/GaSb SQW presented on the main text.

## References


[1] Erlingsson S I and Egues J C 2015 *Phys. Rev. B* **91**(3) 035312

[2] Bernevig B A, Hughes T L and Zhang S C 2006 *Science* **314** 1757–1761

[3] Sai-Halasz G, Esaki L and Harrison W 1978 *Physical Review B* **18** 2812

[4] Yang M, Yang C, Bennett B and Shanabrook B 1997 *Physical Review Letters* **78** 4613

[5] Tsay S F, Chiang J C, Chau Z M and Lo I 1997 *Physical Review B* **56** 13242–13251

[6] Krishtopenko S S and Teppe F 2018 *Science Advances* **4** 4–7

[7] Lakrimi M, Khym S, Nicholas R, Symons D, Peeters F, Mason N and Walker P 1997 *Physical Review Letters* **79** 3034

[8] Nicholas R, Lakrimi M, Khym S, Mason N, Poulter A, Vaughan T, Walker P, Maude D, Portal J, Symons D *et al.* 1998 *Physica B: Condensed Matter* **256** 207–214

[9] Qu F, Beukman A J, Nadj-Perge S, Wimmer M, Nguyen B M, Yi W, Thorp J, Sokolich M, Kiselev A A, Manfra M J *et al.* 2015 *Physical Review Letters* **115** 036803

[10] Hu L H, Liu C X, Xu D H, Zhang F C and Zhou Y 2016 *Physical Review B* **94** 045317

[11] Li J, Yang W and Chang K 2009 *Physical Review B* **80** 035303

[12] Xu W, Li L, Dong H, Gumbs G and Folkes P 2010 *Journal of Applied Physics* **108** 053709

[13] Knez I, Du R R and Sullivan G 2011 *Physical Review Letters* **107** 136603

[14] Suzuki K, Harada Y, Onomitsu K and Muraki K 2013 *Physical Review B* **87** 235311

[15] Nichele F, Pal A N, Pietsch P, Ihn T, Ensslin K, Charpentier C and Wegscheider W 2014 *Physical Review Letters* **112** 036802

[16] Spanton E M, Nowack K C, Du L, Sullivan G, Du R R and Moler K A 2014 *Physical Review Letters* **113** 026804

[17] Du L, Knez I, Sullivan G and Du R R 2015 *Physical Review Letters* **114** 096802

[18] Pribiag V S, Beukman A J, Qu F, Cassidy M C, Charpentier C, Wegscheider W and Kouwenhoven L P 2015 *Nature Nanotechnology* **10** 593

[19] Mueller S, Pal A N, Karalic M, Tschirky T, Charpentier C, Wegscheider W, Ensslin K and Ihn T 2015 *Physical Review B* **92** 081303

[20] Karalic M, Mueller S, Mittag C, Pakrouski K, Wu Q, Soluyanov A A, Troyer M, Tschirky T, Wegscheider W, Ensslin K *et al.* 2016 *Physical Review B* **94** 241402

[21] Nichele F, Suominen H J, Kjaergaard M, Marcus C M, Sajadi E, Folk J A, Qu F, Beukman A J, de Vries F K, van Veen J *et al.* 2016 *New Journal of Physics* **18** 083005

[22] Nguyen B M, Kiselev A A, Noah R, Yi W, Qu F, Beukman A J, de Vries F K, van Veen J, Nadj-Perge S, Kouwenhoven L P *et al.* 2016 *Physical Review Letters* **117** 077701

[23] Kononov A, Kostarev V, Semyagin B, Preobrazhenskii V,

Putyato M, Emelyanov E and Deviatov E 2017 *Physical Review B* **96** 245304

[24] Mueller S, Mittag C, Tschirky T, Charpentier C, Wegscheider W, Ensslin K and Ihn T 2017 *Physical Review B* **96** 075406

[25] Beukman A J, De Vries F K, Van Veen J, Skolasinski R, Wimmer M, Qu F, De Vries D T, Nguyen B M, Yi W, Kiselev A A *et al.* 2017 *Physical Review B* **96** 241401

[26] Skolasinski R, Pikulin D I, Alicea J and Wimmer M 2017 *ArXiv e-prints* (*Preprint* 1709.04830)

[27] Jiang Y, Thapa S, Sanders G, Stanton C, Zhang Q, Kono J, Lou W, Chang K, Hawkins S, Klem J *et al.* 2017 *Physical Review B* **95** 045116

[28] Li C A, Zhang S B and Shen S Q 2018 *Physical Review B* **97** 045420

[29] Zakharova A, Yen S and Chao K A 2002 *Physical Review B* **66** 085312

[30] Lapushkin I, Zakharova A, Yen S and Chao K A 2004 *Journal of Physics: Condensed Matter* **16** 4677

[31] Du L, Li T, Lou W, Wu X, Liu X, Han Z, Zhang C, Sullivan G, Ikhlassi A, Chang K and Du R r 2017 *Physical Review Letters* **119** 056803

[32] Nichele F, Kjaergaard M, Suominen H J, Skolasinski R, Wimmer M, Nguyen B M, Kiselev A A, Yi W, Sokolich M, Manfra M J *et al.* 2017 *Physical Review Letters* **118** 016801
